# Supplementary material for: Hired in High Season: Seasonal Labor Demand and Refugee Labor Market Integration
Source: arXiv:2512.17422 source file (2026-06-18)
Supplement: Supplementary file 1 [file appendix_results.tex]

HVUR & -0.005 & 0.000 & -0.002 & 0.008$^{**}$\\
 & (0.005) & (0.002) & (0.004) & (0.004)\\
\midrule
Observations & 476,624 & 1,013,867 & 89,757 & 86,768\\
